# Supplementary material for: Binding energies of excitonic complexes in type-II quantum rings from diffusion quantum Monte Carlo calculations
Source: arXiv:1811.08700 ancillary file (2019-02-21)
Supplement: Supplementary file 1 [file supplemental.pdf]

# Binding Energies of Excitonic Complexes in Type-II Quantum Rings From Diffusion Quantum Monte Carlo Calculations: Supplemental Material

D. M. Thomas, R. J. Hunt, N. D. Drummond, and M. Hayne
*Department of Physics, Lancaster University, Lancaster LA1 4YB, United Kingdom*
(Dated: December 12, 2018)

To construct an electron orbital $\phi_{\rm e}$ with a continuous first derivative surrounding a ring with sharp corners, the space around the ring was divided into eight regions, with the volume inside the ring comprising a ninth. These nine regions are shown in Fig. 1.

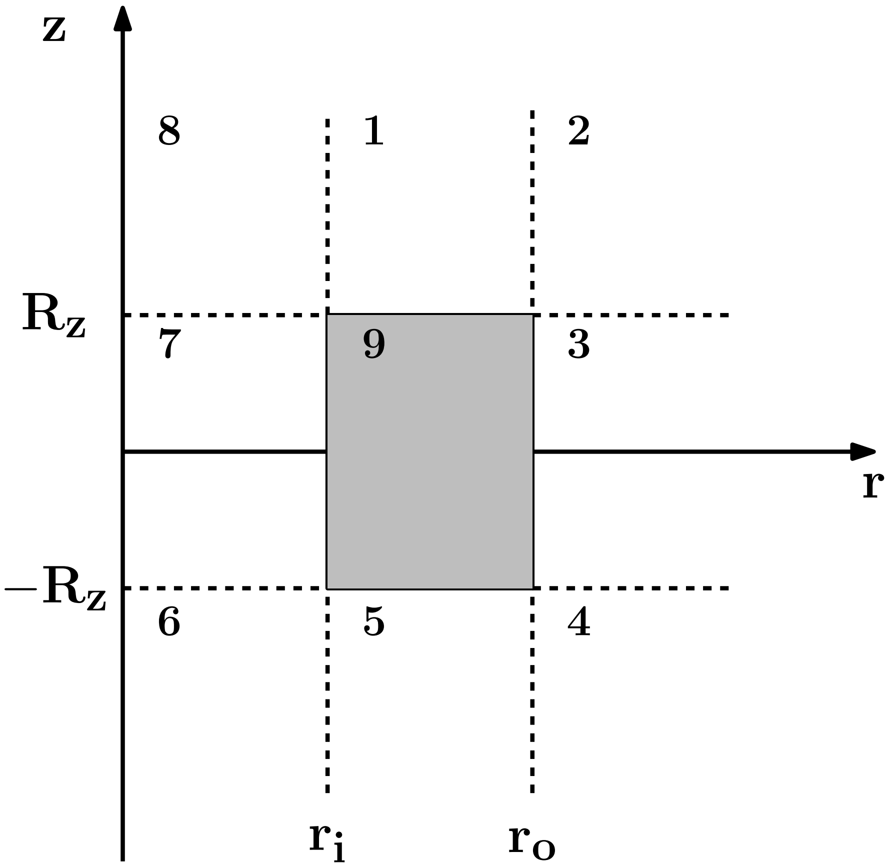


FIG. 1: Nine different regions of space (1–9) used to construct an electron orbital with a continuous first derivative around a quantum ring with a rectangular cross section. $R_z$ is the half-height of the ring, $r_{\rm i}$ is the inner radius, and $r_{\rm o}$ is the outer radius.

The full orbital, for all regions, is then given in cylindrical polar coordinates by

$$\phi_{\rm e}(r,\theta,z) = \begin{cases} \big[a_1(z-R_z)+b_1(z-R_z)^2\big]e^{-\frac{c_1(z-R_z)^2}{1+d_1(z-R_z)}}, & \text{in region 1} \\ \Big[\sqrt{a_1^2(z-R_z)^2+a_3^2(r-r_{\rm o})^2} \\ \qquad +b_1(z-R_z)^2+b_3(r-r_{\rm o})^2\Big]e^{-\sqrt{\frac{c_1^2(z-R_z)^4}{[1+d_1(z-R_z)]^2}+c_3^2(r-r_{\rm o})^2}}, & \text{in region 2} \\ \big[a_3(r-r_{\rm o})+b_3(r-r_{\rm o})^2\big]e^{-c_3(r-r_{\rm o})}, & \text{in region 3} \\ \Big[\sqrt{a_1^2(z+R_z)^2+a_3^2(r-r_{\rm o})^2} \\ \qquad +b_1(z+R_z)^2+b_3(r-r_{\rm o})^2\Big]e^{-\sqrt{\frac{c_1^2(z+R_z)^4}{[1-d_1(z+R_z)]^2}+c_3^2(r-r_{\rm o})^2}}, & \text{in region 4} \\ \big[-a_1(z+R_z)+b_1(z+R_z)^2\big]e^{-\frac{c_1(z+R_z)^2}{1-d_1(z+R_z)}}, & \text{in region 5} \\ \Big[\sqrt{a_1^2(z+R_z)^2+(r_{\rm i}-r)^2(a_7+\frac{a_7 r}{r_{\rm i}}+b_7r^2)^2} \\ \qquad +b_1(z+R_z)^2\Big]e^{-\frac{c_1(z+R_z)^2}{1-d_1(z+R_z)}}, & \text{in region 6} \\ (r_{\rm i}-r)(a_7+\frac{a_7 r}{r_{\rm i}}+b_7r^2), & \text{in region 7} \\ \Big[\sqrt{a_1^2(z-R_z)^2+(r_{\rm i}-r)^2(a_7+\frac{a_7 r}{r_{\rm i}}+b_7r^2)^2} \\ \qquad +b_1(z-R_z)^2\Big]e^{-\frac{c_1(z-R_z)^2}{1+d_1(z-R_z)}}, & \text{in region 8} \\ 0, & \text{in region 9,} \end{cases} \tag{1}$$

where the constants $a_1$, $a_3$, $a_5$, $a_7$, $b_1$, $b_3$, $b_7$, $c_1$, $c_3$, and $d_1$ are variational parameters to be determined by optimization. To ensure correct (i.e., hydrogenic) behavior at long range, it is required that $c_1, c_3, d_1 \geq 0$.
